# Supplementary material for: Integer Multiplier for Orbital Angular Momentum of Light using Circular-Sector Transformation
Source: arXiv:1902.10472 ancillary file (2019-02-27)
Supplement: Supplementary file 1 [file appendix.pdf]

# Integer Multiplier for Orbital Angular Momentum of Light using Circular-Sector Transformation – Supplementary material

Satoru Takashima,[1] Hirokazu Kobayashi,[1, *] and Katsushi Iwashita[1]

[1]*Graduate School of Engineering, Kochi University of Technology, 185 Tosayamada-cho, Kochi 782-8502 Japan*

(Dated: February 27, 2019)

## STATIONARY PHASE METHOD FOR $2f$ CONFIGURATION AND ITS COMPLEX REPRESENTATION

Here we describe stationary phase method for approximating Fresnel diffraction integral in $2f$ system. When the input complex amplitude (scalar electric field) $E_{\mathrm{in}}(\boldsymbol{r})$ at the incident plane $\boldsymbol{r} = (x, y)$ is subjected to the transforming phase $\varphi(\boldsymbol{r})$ and propagated along $z$-direction in $2f$ system, the complex amplitude $E_{\mathrm{out}}(\boldsymbol{s}, z)$ on the plane $\boldsymbol{s} = (u, v)$ at the distance $z$ is calculated by Fresnel diffraction integral as follows

$$E_{\mathrm{out}}(\boldsymbol{s}, z) = \frac{\mathrm{e}^{\mathrm{i}kz}}{\mathrm{i}\lambda z} \int E_{\mathrm{in}}(\boldsymbol{r}) \mathrm{e}^{\mathrm{i}\varphi(\boldsymbol{r})} \mathrm{e}^{\mathrm{i}\frac{k}{2z}|\boldsymbol{r}-\boldsymbol{s}|^2} \mathrm{d}\boldsymbol{r}, \tag{1}$$

where $k$ is the wavenumber and $\lambda$ is the wavelength. Next consider propagation of the light wave after passing through the Fourier transforming lens with the focal length of $f$ placed at $z = f$. When the total propagation distance is $z$, the complex amplitude after the lens can be calculated as

$$E_{\mathrm{out}}(\boldsymbol{s}, z) = \frac{\mathrm{e}^{\mathrm{i}kz}}{\mathrm{i}\lambda f} \int E_{\mathrm{in}}(\boldsymbol{r}) \mathrm{e}^{\mathrm{i}\varphi(\boldsymbol{r})} \exp\left[-\mathrm{i}\frac{k}{f}\left\{\boldsymbol{s}\cdot\boldsymbol{r} - \left(1 - \frac{z}{2f}\right)|\boldsymbol{r}|^2\right\}\right] \mathrm{d}\boldsymbol{r}. \tag{2}$$

When $z = 2f$, Eq. (2) becomes

$$E_{\mathrm{out}}(\boldsymbol{s}, 2f) = \frac{\mathrm{e}^{\mathrm{i}kz}}{\mathrm{i}\lambda f} \int E_{\mathrm{in}}(\boldsymbol{r}) \mathrm{e}^{\mathrm{i}\varphi(\boldsymbol{r})} \exp\left(-\mathrm{i}\frac{k}{f}\boldsymbol{s}\cdot\boldsymbol{r}\right) \mathrm{d}\boldsymbol{r} \tag{3}$$

$$\propto \mathcal{F}\left[E_{\mathrm{in}}(\boldsymbol{r})\right]\left(\frac{k}{f}\boldsymbol{s}\right), \tag{4}$$

where $\mathcal{F}[\cdot]$ represents Fourier transform calculation. Equation (4) shows that the input-output relationship of $2f$ configuration can be formulated by Fourier transform.

The stationary phase method of determining the Fresnel diffraction integral is strictly true only in the limit of infinitely large wavenumber $k$. However, it remains an excellent approximation for appropriate large value of $k$ (small wavelength $\lambda$). This approximation states that the only significant contributions to the integral occur at the points where the phase gradient vanishes, called as the stationary phase point. In approximating Fresnel diffraction integrals of Eqs. (1) and (2) by stationary phase method, the stationary phase point satisfies the following equations

$$\boldsymbol{\nabla}\varphi(\boldsymbol{r}) = \begin{cases} -\dfrac{k}{z}(\boldsymbol{r} - \boldsymbol{s}) & \text{for } \ 0 \le z \le f \\ -\dfrac{k}{f}\left[\left(2 - \dfrac{z}{f}\right)\boldsymbol{r} - \boldsymbol{s}\right] & \text{for } \ f \le z \le 2f \end{cases}, \tag{5}$$

where $\boldsymbol{\nabla} \equiv \left(\frac{\partial}{\partial x}, \frac{\partial}{\partial y}\right)$ is the two-dimensional differential operator. The first and the second equations in Eq. (5) show the stationary phase conditions before and after the Fourier transforming lens, respectively. When $z = 2f$, Eq. (5) becomes

$$\boldsymbol{\nabla}\varphi(\boldsymbol{r}) = \frac{k}{f}\boldsymbol{s}. \tag{6}$$

For applications of geometric transformation, a mapping $\boldsymbol{r} = (x, y) \mapsto \boldsymbol{s}(\boldsymbol{r}) = (u(x, y), v(x, y))$ is given, and the partial differential equation in Eq. (6) is solved for $\varphi(\boldsymbol{r})$. Assuming that $u(x, y)$ and $v(x, y)$ have partial derivatives in a simply connected region at the input plane, Eq. (6) have solutions for $\varphi(\boldsymbol{r})$ only when the following continuity condition is satisfied,

$$\frac{\partial u}{\partial y} = \frac{\partial v}{\partial x} \tag{7}$$

or equivalently,

$$\frac{\partial\varphi}{\partial x\partial y}=\frac{\partial\varphi}{\partial y\partial x}. \tag{8}$$

By the stationary phase method, the Fresnel diffraction integral in Eq. (3) can be approximated as

$$E_{\text{out}}(\boldsymbol{s},2f)\simeq\frac{2\pi\sigma\mathrm{e}^{\mathrm{i}2kf}}{\mathrm{i}\lambda f\sqrt{|\varphi_{xx}\varphi_{yy}-\varphi_{xy}^2|}}E_{\text{in}}(\boldsymbol{r}_0)\exp\left[\mathrm{i}\left\{\varphi(\boldsymbol{r}_0)-\frac{k}{f}\boldsymbol{r}_0\cdot\boldsymbol{s}\right\}\right], \tag{9}$$

where $\boldsymbol{r}_0$ is the stationary point, the notation $\varphi_{xx}=\partial^2\varphi/\partial x^2$, etc., is used, and $\sigma$ is defined by

$$\sigma=\begin{cases}\mathrm{i} & \text{for } \varphi_{xx}>0, \varphi_{xx}\varphi_{yy}>\varphi_{xy}^2\\ -\mathrm{i} & \text{for } \varphi_{xx}<0, \varphi_{xx}\varphi_{yy}>\varphi_{xy}^2\\ 1 & \text{for } \varphi_{xx}\varphi_{yy}<\varphi_{xy}^2\end{cases}. \tag{10}$$

From Eq. (9), the correction phase $\Psi(\boldsymbol{s})$ for compensating the undesired phase term is given by

$$\Psi(\boldsymbol{s})=-\varphi(\boldsymbol{r}_0)+\frac{k}{f}\boldsymbol{r}_0\cdot\boldsymbol{s}. \tag{11}$$

Now we consider the geometric transformation as the coordinate mapping in complex planes from $\zeta=x+\mathrm{i}y$ to $\omega=u+\mathrm{i}v$. In what follows, the complex variable $\omega$ is written as $\omega(z)$ to explicitly indicate the dependence on propagation distance $z$ and the transforming phase is written in complex form as $\varphi(\zeta,\bar{\zeta})$, where $\bar{\zeta}=x-\mathrm{i}y$. Then, the stationary phase condition in Eq. (5) can be given in complex form as follows

$$\frac{\partial\varphi(\zeta,\bar{\zeta})}{\partial\bar{\zeta}}=\begin{cases}-\dfrac{k}{2z}\left[\zeta-\omega(z)\right] & \text{for } 0\le z\le f\\ -\dfrac{k}{2f}\left[\left(2-\dfrac{z}{f}\right)\zeta-\omega(z)\right] & \text{for } f\le z\le 2f\end{cases}, \tag{12}$$

where $\frac{\partial}{\partial\bar{\zeta}}$ is called as the Wirtinger operator and defined as

$$\frac{\partial}{\partial\bar{\zeta}}=\frac{1}{2}\left(\frac{\partial}{\partial x}+\mathrm{i}\frac{\partial}{\partial y}\right). \tag{13}$$

When $z=2f$, Eq. (12) becomes

$$\frac{\partial\varphi(\zeta,\bar{\zeta})}{\partial\bar{\zeta}}=\frac{k}{2f}\omega(2f). \tag{14}$$

In the complex function theory, the continuity condition in Eq. (7) can be satisfied by anti-analytic function $g(\bar{\zeta})$, which depends only on $\bar{\zeta}$ not on $\zeta$. The anti-analytic function $g(\bar{\zeta})=u(x,y)+\mathrm{i}v(x,y)$ satisfies the following Cauchy-Riemann equation,

$$\frac{\partial u}{\partial x}=-\frac{\partial v}{\partial y}, \tag{15}$$

$$\frac{\partial u}{\partial y}=\frac{\partial v}{\partial x}, \tag{16}$$

where the second equation is equal to the continuity condition. Thus, we consider the anti-analytic function $g(\bar{\zeta})$ as coordinate mapping at $z=2f$, i.e., $\omega(2f)=g(\bar{\zeta})$. The stationary phase condition at $z=2f$ is formulated as

$$\frac{\partial\varphi(\zeta,\bar{\zeta})}{\partial\bar{\zeta}}=\frac{k}{2f}g(\bar{\zeta}). \tag{17}$$

From Eq. (17) and its complex conjugate, the solution can be expressed as a simple form given by

$$\varphi(\zeta,\bar{\zeta})=\frac{k}{f}\mathrm{Re}\left[\int g(\bar{\zeta})\mathrm{d}\bar{\zeta}\right]. \tag{18}$$

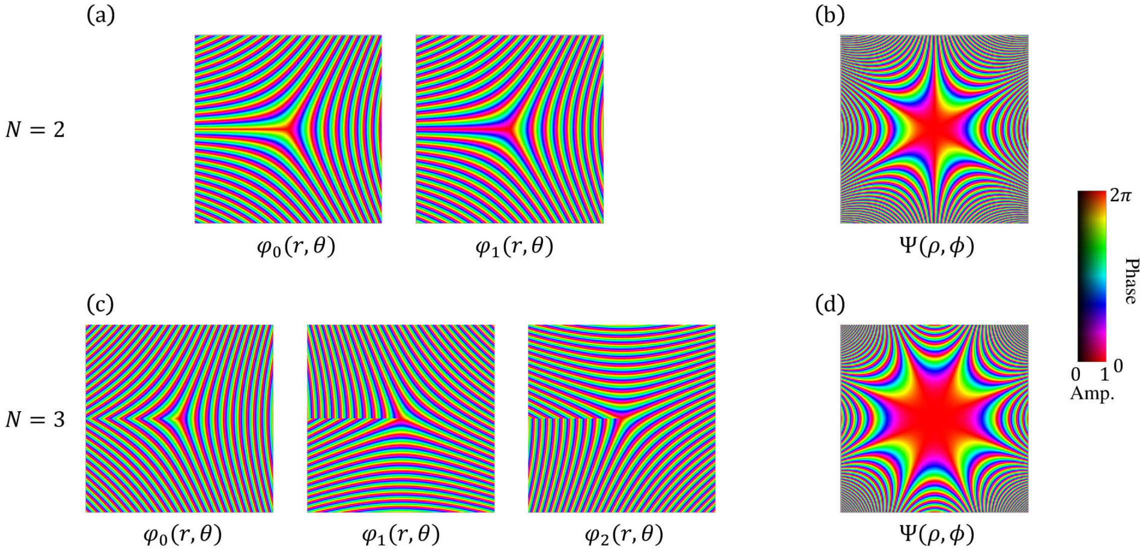


FIG. 1: Required transforming phases $\varphi_n(r,\theta)$ and the correction phase $\Psi(\rho,\phi)$ for the OAM doubler [(a),(b)] and for the OAM tripler [(c),(d)].

The correction phase $\Psi(\boldsymbol{s})$ in Eq. (11) can be also written in complex form as

$$\Psi(\omega,\bar{\omega}) = -\varphi(\zeta_0,\bar{\zeta}_0) + \frac{k}{f}\mathrm{Re}\left[\omega\bar{\zeta}_0\right], \tag{19}$$

where $\zeta_0$ and $\bar{\zeta}_0$ represent the stationary phase point. Moreover, from Eqs. (12) and (17), the ideal conversion process of the coordinate system under propagation inside $2f$ system can be simply represented by

$$\omega(z) = \begin{cases} \zeta + \dfrac{z}{f}g(\bar{\zeta}) & \text{for } \ 0 \le z \le f \\ \left(2-\dfrac{z}{f}\right)\zeta + g(\bar{\zeta}) & \text{for } \ f \le z \le 2f \end{cases}. \tag{20}$$

As a specific example, we consider a fractional power function $g(\bar{\zeta}) = \alpha\bar{\zeta}^{\frac{1}{N}}$ with the multiplier factor $N$ and the scaling constant $\alpha$ as an anti-analytic complex function. The fractional power function is a $N$-valued function, and thus $N$ number of transforming phases $\varphi_n$ with integer $n = 0,\cdots,N-1$ are obtained from Eq. (18). From Eqs. (18) and (19), the transforming phase on the polar coordinate $\zeta = r\mathrm{e}^{\mathrm{i}\theta}$ and the correction phase on the polar coordinate $\omega = \rho\mathrm{e}^{\mathrm{i}\phi}$ is given by

$$\varphi_n(r,\theta) = \frac{\alpha k}{f}\frac{Nr^{1+\frac{1}{N}}}{N+1}\cos\left[\frac{(N+1)\,\theta + 2n\pi}{N}\right], \tag{21}$$

$$\Psi(\rho,\phi) = \frac{k}{f}\left(\frac{\rho}{|\alpha|}\right)^N \left[\frac{\rho\ \cos\left[(N+1)\,\phi\right]}{N+1}\right]. \tag{22}$$

Figure 1 shows the required phase distributions for the OAM doubler ($N = 2$) and tripler ($N = 3$). Moreover, by substituting $g(\bar{\zeta})$ to Eq. (20), the ideal conversion process of the polar coordinates can be obtained, as shown in Fig. 2. Each coordinate mapping with the particular value of $n$ converts the circular shape of the input OAM mode to the circular-sector shape at the different azimuthal position depending on $n$.

## COMPLEX AMPLITUDE MODULATION BY PHASE-ONLY SPATIAL LIGHT MODULATOR

Here we describe a method to implement complex phase modulation by using a single phase-only spatial light modulator (SLM). Let $A(\boldsymbol{r})\mathrm{e}^{\mathrm{i}\varphi(\boldsymbol{r})}$ be the complex amplitude modulation, where $A(\boldsymbol{r})$ and $\varphi(\boldsymbol{r})$ represent normalized

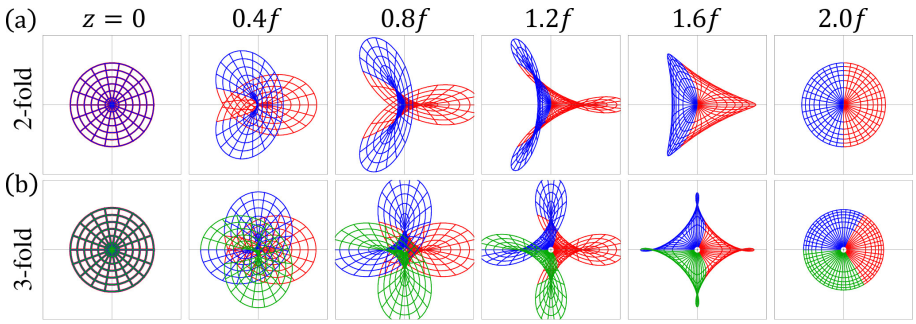


FIG. 2: Ideal conversion process of the two and the three polar coordinates (red, blue, and green) by OAM multiplication with $N = 2$ (OAM doubler) and $N = 3$ (OAM tripler).

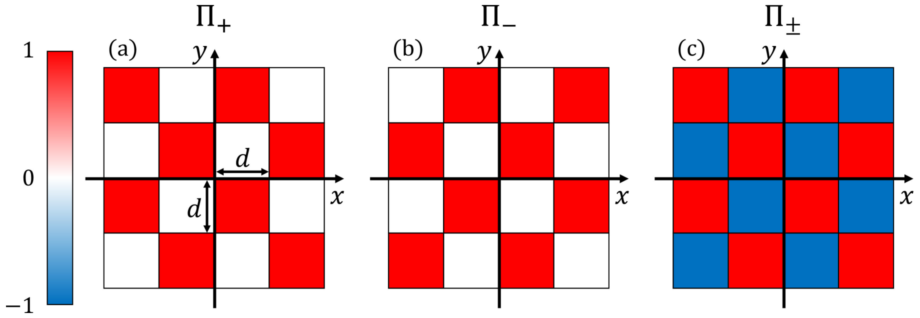


FIG. 3: Mutually-complementary checkerboard patterns, (a) $\Pi_+(\boldsymbol{r})$, (b) $\Pi_-(\boldsymbol{r})$, and (c) $\Pi_\pm(\boldsymbol{r}) \equiv \Pi_+(\boldsymbol{r}) - \Pi_-(\boldsymbol{r})$.

amplitude and phase distribution, respectively. This modulation can be written as the sum of two phase only modulation,

$$A(\boldsymbol{r})\mathrm{e}^{\mathrm{i}\varphi(\boldsymbol{r})} = \frac{1}{2}\left\{\mathrm{e}^{\mathrm{i}P_+(\boldsymbol{r})} + \mathrm{e}^{\mathrm{i}P_-(\boldsymbol{r})}\right\}, \tag{23}$$

where two phase distributions, $P_+(\boldsymbol{r})$ and $P_-(\boldsymbol{r})$ are defined as

$$P_\pm(\boldsymbol{r}) = \varphi(\boldsymbol{r}) \pm \cos^{-1} A(\boldsymbol{r}). \tag{24}$$

In order to realize Eq. (23) by using the single phase-only SLM with pixel size $d$, we consider the following phase only modulation,

$$\mathrm{e}^{\mathrm{i}\Phi(\boldsymbol{r})} = \Pi_+(\boldsymbol{r})\mathrm{e}^{\mathrm{i}P_+(\boldsymbol{r})} + \Pi_-(\boldsymbol{r})\mathrm{e}^{\mathrm{i}P_-(\boldsymbol{r})}, \tag{25}$$

where $\Pi_+(\boldsymbol{r})$ and $\Pi_-(\boldsymbol{r})$ are mutually complementary functions satisfying $\Pi_+(\boldsymbol{r}) + \Pi_-(\boldsymbol{r}) = 1$, and they are spatially periodic functions giving 0 or +1 with period $2d$, like a two-dimensional binary gratings [checker-board patterns as shown in Fig. 3(a) and (b)]. The phase distribution $\Phi(\boldsymbol{r})$ in Eq. (25) is formulated as

$$\begin{aligned}\Phi(\boldsymbol{r}) &= P_+(\boldsymbol{r})\Pi_+(\boldsymbol{r}) + P_-(\boldsymbol{r})\Pi_-(\boldsymbol{r}) \\ &= \varphi(\boldsymbol{r}) + \Pi_\pm(\boldsymbol{r})\cos^{-1} A(\boldsymbol{r})\end{aligned} \tag{26}$$

where $\Pi_\pm(\boldsymbol{r}) \equiv \Pi_+(\boldsymbol{r}) - \Pi_-(\boldsymbol{r})$ is spatially periodic function giving +1 or −1 [see Fig. 3(c)]. The Fourier series expansion of $\Pi_+$ and $\Pi_-$ are given by

$$\Pi_+(\boldsymbol{r}) = \frac{1}{2} + \sum_{n,m\neq 0} c_{n,m}\mathrm{e}^{\mathrm{i}\frac{\pi}{d}(nx+my)}, \tag{27}$$

$$\Pi_-(\boldsymbol{r}) = \frac{1}{2} - \sum_{n,m\neq 0} c_{n,m}\mathrm{e}^{\mathrm{i}\frac{\pi}{d}(nx+my)}, \tag{28}$$

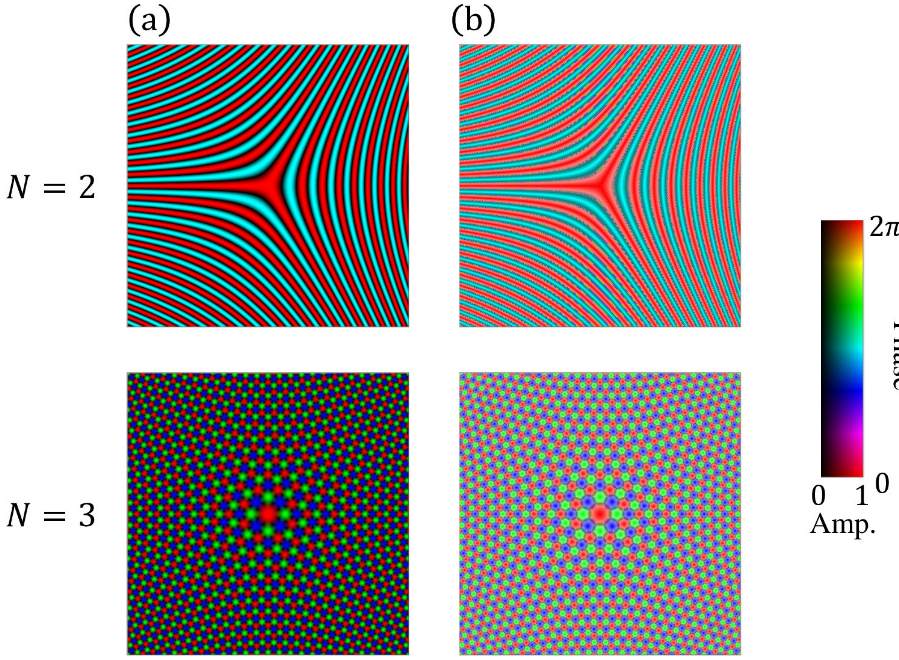


FIG. 4: Required amplitude and phase modulation for the OAM multiplier with $N = 2$ (OAM doubler) and $N = 3$ (OAM tripler). (a) Complex amplitude modulation $A(\boldsymbol{r})\mathrm{e}^{\mathrm{i}\varphi(\boldsymbol{r})}$. (b) Phase only modulation to achieve the complex amplitude modulation.

where

$$c_{n,m} = \frac{\{(-1)^n - 1\}\{(-1)^m - 1\}}{2nm\pi^2}. \tag{29}$$

The Fourier transform of the phase-only modulation in Eq. (25) with respect to $\boldsymbol{r} = (x, y)$ is calculated as

$$\mathcal{F}\left[\mathrm{e}^{\mathrm{i}\Phi(\boldsymbol{r})}\right] = \mathcal{F}\left[\Pi_+(\boldsymbol{r})\right] * \mathcal{F}\left(\mathrm{e}^{\mathrm{i}P_+(\boldsymbol{r})}\right) + \mathcal{F}\left[\Pi_-(\boldsymbol{r})\right] * \mathcal{F}\left(\mathrm{e}^{\mathrm{i}P_-(\boldsymbol{r})}\right) \tag{30}$$

$$= \frac{1}{2}\mathcal{F}\left[\mathrm{e}^{\mathrm{i}P_+(\boldsymbol{r})} + \mathrm{e}^{\mathrm{i}P_-(\boldsymbol{r})}\right](k_x, k_y) + \sum_{n,m\neq 0} c_{n,m}\mathcal{F}\left[\mathrm{e}^{\mathrm{i}P_+(\boldsymbol{r})} - \mathrm{e}^{\mathrm{i}P_-(\boldsymbol{r})}\right]\left(k_x - \frac{n\pi}{d}, k_y - \frac{m\pi}{d}\right), \tag{31}$$

where $k_x$ and $k_y$ are two components of spatial angular frequency or wavenumber. Thus, the complex amplitude modulation in Eq. (23) can be achieved by applying a spatial low-pass filter to extract the first term in from Eq. (31) (zeroth-order diffraction component). This method is called as the double-phase hologram technique.

Figure 4(a) and (b) show the required complex amplitude modulation for the OAM multiplier with $N = 2, 3$ and their double-phase hologram on the phase-only SLM, respectively. Figure 4(a) has both the amplitude (brightness) and the phase (hue) distributions, while Fig. 4(b) has only phase distribution and its amplitude is uniform.

## MEASUREMENT METHOD OF COMPLEX AMPLITUDE DISTRIBUTION

In this section, we describe about angular spectrum method to extract complex amplitude from interference pattern. Let $E_l(\boldsymbol{r})$ be complex amplitude of OAM mode with topological charge $l$. The intensity distribution $I(\boldsymbol{r})$ of the interference pattern between the OAM mode $E_l(\boldsymbol{r})$ propagating along $z$ direction and the reference beam $E_0(\boldsymbol{r})$ with slightly tilted angle $\Theta$ from $z$ axis can be calculated as

$$I(\boldsymbol{r}) \equiv \left|E_0(\boldsymbol{r})\mathrm{e}^{\mathrm{i}xk\sin\Theta} + E_l(\boldsymbol{r})\right|^2$$

$$= \left|E_0(\boldsymbol{r})\right|^2 + \left|E_l(\boldsymbol{r})\right|^2 + \bar{E}_0(\boldsymbol{r})E_l(\boldsymbol{r})\mathrm{e}^{-\mathrm{i}xk\sin\Theta} + \text{c.c.}, \tag{32}$$

where $k$ is the wavenumber, $\bar{E}_0(\boldsymbol{r})$ is the complex conjugate of $E_0(\boldsymbol{r})$, and c.c. represents complex conjugate of the previous term. The last two terms in Eq. (32) are interference terms. The Fourier transform of the interference terms

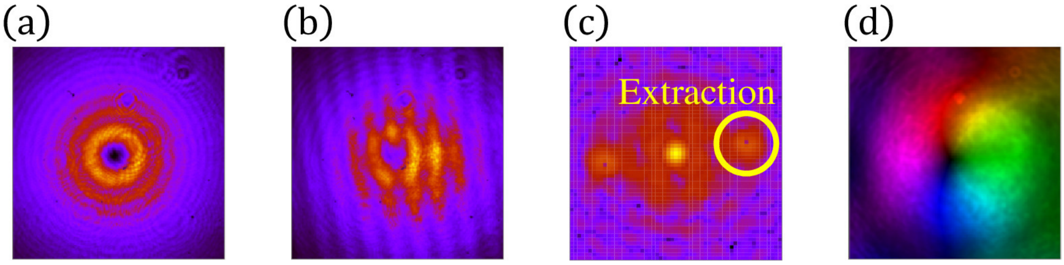


FIG. 5: (a) Intensity distribution of the OAM mode with $l = 1$. (b) Interference pattern between the OAM mode with $l = 1$ and the reference beam. (c) Fourier transform intensity of the interference pattern. (d) Optical complex amplitude extracted from one of shifted interference term in angular spectrum domain.

can be formulated as

$$\mathcal{F}\left[\bar{E}_0(\boldsymbol{r})E_l(\boldsymbol{r})\right](k_x + k\sin\Theta) + \mathcal{F}\left[E_0(\boldsymbol{r})\bar{E}_l(\boldsymbol{r})\right](k_x - k\sin\Theta). \tag{33}$$

Thus, the interference terms are shifted by amount of $\pm k\sin\Theta$ in angular spectrum domain. If the spatial variations of $E_0(\boldsymbol{r})$ and $E_l(\boldsymbol{r})$ are slow compared with the spatial angular frequency $k\sin\Theta$, we can isolate the angular spectrum corresponding to $\bar{E}_0(\boldsymbol{r})E_l(\boldsymbol{r})$. We translate the isolated interference term by $k\sin\Theta$ along $k_x$ axis on the angular spectrum domain and calculate the inverse Fourier transform of the translated term. Finally, the result of inverse Fourier transform is divided by the experimentally-obtained amplitude $|E_0|$ of the reference beam and desired complex amplitude $E_l(\boldsymbol{r})$ can be obtained. It is noticed that the calculated result includes the phase distribution of the reference beam $E_0(\boldsymbol{r})$. Thus, this method is suitable for the interference pattern with a quasi plane wave as reference beam.

Figure 5 shows an calculation example. Figure 5(a) is experimentally-obtained intensity distribution of the OAM mode with $l = 1$ and Fig. 5(b) is the interference pattern between the OAM mode with $l = 1$ and the reference beam. By calculating fast Fourier transformation, we obtain the angular spectrum distribution, as shown in Fig. 5(c). By extracting one of shifted components in the angular spectrum domain and performing inverse Fourier transform, we can reconstruct the complex amplitude of the OAM mode, as shown in Fig. 5(d).

## CALCULATION OF OAM SPECTRUM

Here we describe how to analyze the OAM spectrum from the complex amplitude distribution $E(r,\theta)$ with radius $r$ and azimuthal angle $\theta$ on the polar coordinate system. Since $E(r,\theta)$ is a periodic function with respect to $\theta$, it can be expressed as Fourier series expansion for $\theta$ as follows,

$$E(r,\theta) = \sum_{l=-\infty}^{\infty} C_l(r)\mathrm{e}^{\mathrm{i}l\theta}, \tag{34}$$

$$C_l(r) = \frac{1}{2\pi}\int_{-\pi}^{\pi} E(r,\theta)\mathrm{e}^{-\mathrm{i}l\theta}\mathrm{d}\theta. \tag{35}$$

From the Parseval's theorem, the following equation is valid,

$$\frac{1}{2\pi}\int_{-\pi}^{\pi}|E(r,\theta)|^2\,\mathrm{d}\theta = \sum_{l=-\infty}^{\infty}|C_l(r)|^2. \tag{36}$$

Thus, the total intensity $I_{\mathrm{total}}$ is obtained by

$$I_{\mathrm{total}} = \int_0^{\infty}\int_{-\pi}^{\pi}|E(r,\theta)|^2\,r\mathrm{d}r\mathrm{d}\theta = \sum_{l=-\infty}^{\infty}2\pi\int_0^{\infty}|C_l(r)|^2\,r\mathrm{d}r. \tag{37}$$

The intensity $I_l$ of the OAM mode with the topological charge $l$ can be defined as

$$I_l \equiv 2\pi\int_0^{\infty}|C_l(r)|^2\,r\mathrm{d}r. \tag{38}$$

The intensity ratio or probability $P_l$ of the OAM mode $l$ is expressed as

$$P_l \equiv \frac{I_l}{I_{\text{total}}}. \tag{39}$$

The averaged OAM value $\langle l \rangle$ and its standard deviation $\delta l$ can be calculated as

$$\langle l \rangle = \sum_l l P_l, \tag{40}$$

$$\delta l = \sqrt{\sum_l \left(l - \langle l \rangle\right)^2 P_l}. \tag{41}$$

The experimentally-obtained complex amplitude is slowly-varying discrete data set. Thus, by using interpolation function, it is possible to estimate the complex amplitude function $E(r, \theta)$ at an arbitrary point $(r, \theta)$ on the polar coordinate. In our manuscript, the averaged OAM $\langle l \rangle$ and its standard deviation $\delta l$ is calculated within the range of $-10 \leq l \leq 10$ by using Eqs. (40) and (41).

---

* Electronic address: kobayashi.hirokazu@kochi-tech.ac.jp
